# Supplementary material for: Improving Molecular Design by Stochastic Iterative Target Augmentation
Source: arXiv:2002.04720 source file (2021-08-15)
Supplement: Supplementary file 1 [file old_appendix_sections.tex]

% \subsection{Ablation}

% We conduct some ablation experiments for our output-filtering framework for the VSeq2Seq base architecture in the molecular optimization setting. 

% We experiment with Vseq2seq(test), a version of our model that does not use the external filter with output-filtering to augment the data during training. Instead, it merely uses the external filter to filter the outputs of the base model at test time. As shown in Table \ref{tab:ablation}, Vseq2seq(test) performs significantly worse than our model Vseq2seq+ with the full output-filtering framework. Similarly, a model Vseq2seq(train) with only the data augmentation but without the prediction-time filtering also underperforms. 

% In a separate experiment, we run a self-training-only version of the model. This model augments the data in each output-filtering epoch by simply using the first $K$ new translations for each training set precursor, without using the external filter at all. We find that the performance of this model steadily declines from that of the bootstrapped starting point with each output-filtering epoch, indicating that the external filter is necessary to prevent poor data from leading the model training astray. 

% % \begin{table}[]
% % \centering
% % \begin{tabular}{|l|l|l|l|l|}
% % \hline
% % Model                        & QED Success & QED Diversity & DRD2 Success & DRD2 Diversity \\ \hline
% % Vseq2seq                     & 58.5        & 0.331         & 75.9         & 0.176          \\ \hline
% % Vseq2seq + test time filter  & 69.3        & 0.421         & 87.2         & 0.2            \\ \hline
% % Vseq2seq + train time filter & 81.8        & 0.43          & 92.2         & 0.321          \\ \hline
% % Vseq2seq + augment           & 89          & 0.47          & 97.2         & 0.361          \\ \hline
% % \end{tabular}
% % \caption{Ablation analysis of filtering at training and test time.}
% % \label{tab:ablation}
% % \end{table}

% \begin{table}[]
% \begin{tabular}{|l|l|l|l|l|l|l|}
% \hline
% Model            & Train filter & Test filter & QED Suc. & QED Div. & DRD2 Suc. & DRD2 Div. \\ \hline
% Vseq2seq         & {\color{red}\xmark }               & {\color{red}\xmark }                        & 58.5        & 0.331         & 75.9         & 0.176          \\\hline
% \textit{Vseq2seq (test)}  &{\color{red}\xmark }               & {\color{green}\cmark }                       & 69.3        & 0.421         & 87.2         & 0.200            \\\hline
% \textit{Vseq2seq (train)} & {\color{green}\cmark }               & {\color{red}\xmark }                        & 81.8        & 0.43          & 92.2         & 0.321          \\\hline
% \textit{Vseq2seq+}        & {\color{green}\cmark }               & {\color{green}\cmark }                       & 89          & 0.47          & 97.2         & 0.361         \\\hline
% \end{tabular}
% \caption{Ablation analysis of filtering at training and test time. ``Train filter" indicates a model whose training process underwent data augmentation according to our output-filtering framework. ``Test filter" indicates a model that used the external filter at prediction time to discard candidate outputs that did not pass the external filter.}
% \label{tab:ablation}
% \end{table}

% TODO same table for code generation task if time allows, and maybe other experiments of interest for molecule setting
\iffalse

\section{Iterative vs. Idealized Scenario for Model Training} \label{iterative_idealized}

As mentioned in Section \ref{theory}, we now show that the iterative E-M approach may converge to a different, higher-performing optimum than in the idealized direct projection case. 

Consider a scenario where we now drop the assumption that our model is arbitrarily powerful, and consider the following toy problem with a very limited model. Our model $P(Y|X)$ generates a one-dimensional output independent of $X$, distributed according to an $N(\mu, 1)$ Gaussian with a single parameter $\mu$. Suppose $\mu$ is initialized to $0$, and that our target region $B(X)$ is the region $Y > 0$. Directly projecting our initial distribution onto the output results in the distribution on the left of Figure \ref{fig:gaussian}, while iteratively updating $\mu$ according to training examples from the region $B(X)$ results in shifting the distribution to the right, for example as depicted in the right side of Figure \ref{fig:gaussian}. It is clear that the latter distribution is different from the former. In fact, it achieves a higher mean $Y$ --- which in a task like molecular optimization could be interpreted as ``property score" --- compared to the resulting distribution from the direct projection. By contrast, the direct projection results in a distribution where much of the probability mass lies near the boundary of the space of desired outcomes. In a scenario like molecular optimization where we might prefer higher property score, we hypothesize that a similar phenomenon may benefit our iterative E-M approach. 

\begin{figure*}[hbt!]
    \centering
    \begin{subfigure}[t]{0.475\textwidth}
        \centering
        \includegraphics[height=1.6in]{figures/base_gaussian.png}
        % \caption{}
        \label{fig:gaussiana}
    \end{subfigure}%
    \hfill
    \begin{subfigure}[t]{0.475\textwidth}
        \centering
        \includegraphics[height=1.6in]{figures/iterative_gaussian.png}
        % \caption{}
        \label{fig:gaussianb}
    \end{subfigure}
    \caption{\textbf{Left}: Direct projection of the Gaussian onto the region $Y > 0$ (projected distribution in dark blue). \textbf{Right}: Projection of the Gaussian resulting from iterative updates onto the region $Y > 0$. The shifted Gaussian from iterative updates has a greater mean $Y$ compared to the direct projection. }
    \label{fig:gaussian}
\end{figure*}

We now substantiate this intuitive argument by conducting an experiment, although the difference is small.

\begin{table}[hbt!]
\centering
\begin{tabular}{|l|l|l|l|l|}
\hline
\textbf{Model}    & \textbf{QED Success} & \textbf{QED Diversity} & \textbf{DRD2 Success} & \textbf{DRD2 Diversity} \\ \Xhline{1.6pt}
Vseq2seq+         &    89.0                  &   0.470                     &    97.2                   &   0.361                      \\ \hline
Vseq2seq+(Ideal) &   88.8                   &    0.476                    &     96.4                  &     0.354                    \\ \hline
\end{tabular}
\caption{Iterative E-M approach vs Direct Projection (``Ideal") approach.}
\label{tab:iterative_ideal}
\end{table}

For both the QED and DRD2 tasks, we run our VSeq2Seq+ model as usual. We compute the total number of distinct translations generated over the course of training for each precursor molecule, which pass the external filter. Let $K'$ be the average number of distinct translations per input (rounded to the nearest integer). We run an alternative version of our model, VSeq2Seq+(Ideal), which bootstraps the model as normal using the original training data, and then generates $K'$ distinct translations per precursor molecule. We set $C = 2000$ so that the model finds $K'$ successful translations for virtually all precursor molecules. VSeq2Seq+(Ideal) then trains to convergence on this training dataset, without generating any more new targets; it can thus be viewed as a non-iterative version of our method. This implementation of a direct projection approach eventually nears the performance of the iterative EM approach we adopt in the paper, as shown in Table \ref{tab:iterative_ideal}. However, the direct projection approach requires significantly more training steps to converge, and repeating the experiment reproduces the small gap in success rate between the models. 


\section{Discussion of Domain Applicability}\label{domain_app} % TODO move most of it to appendix

We discuss the relative importance of different features of our molecular optimization tasks, providing insight into the domains where our iterative target augmentation approach may be useful. %We first analyze the influence of the quality of the property predictor used to evaluate candidate translations, by rerunning our experiments with inferior predictors (obtained by training weaker models, simulating the situation where a property is difficult to learn). Predictor quality is measured by RMSE with the ground truth model on the test set. 

% \begin{figure*}[hbt!]
%     \centering
%     \begin{subfigure}[t]{0.475\textwidth}
%         \centering
%         \includegraphics[height=1.6in]{figures/qed_predictor.pdf}
%     \end{subfigure}%
%     \hfill
%     \begin{subfigure}[t]{0.475\textwidth}
%         \centering
%         \includegraphics[height=1.6in]{figures/drd2_predictor.pdf}
%     \end{subfigure}
%     \vspace{-5pt}
%     \caption{\textbf{Left}: QED success rate vs. RMSE of the Chemprop predictor against the ground truth on the test set. \textbf{Right}: Same plot for DRD2. For each plot, the far left point with zero RMSE is obtained by reusing the ground truth predictor, while the second-from-left point on each plot is the Chemprop predictor we use to obtain our main results.}
%     \label{fig:pred_rmse}
% \end{figure*}

As shown in Figure \ref{fig:pred_rmse} in the main text, although QED and DRD2 are not the most challenging endpoints to model \textit{in silico}, we maintain strong performance even when using greatly inferior property predictors in our external filter. This indicates that iterative target augmentation can be viable for tasks with weaker property predictors as well. We note that accurate ground truth evaluation for difficult-to-model properties may be cumbersome, potentially requiring laboratory experiments. It could be time-consuming and expensive to calculate metrics to quantify model performance. However, this evaluation issue does not preclude our model from generating helpful suggestions to a medicinal chemist in a practical use scenario.

In principle, iterative target augmentation is applicable to many domains outside of molecular optimization and program synthesis. For example, if the external filter is a binary sentiment classifier, one can use the framework for sentiment classification. If we can predict whether two sentences in different languages have the same semantic meaning, then the framework can be used for machine translation. In short, the external filter merely predicts whether a source-target pair is valid, however that is defined. 

In fact, a similar iterative target augmentation approach is possible even in tasks where each input corresponds to only a single correct output, as long as additional unlabeled precursors are provided as in the semi-supervised setting. 

However, some tasks have practical issues to resolve before transferring the method becomes feasible. For instance, it is trivial to check whether a molecule is well-formed, but this is more difficult in natural language. Thus it may be necessary for the external filter to include a grammar checking component in natural language tasks. 

Finally, one may be concerned about the computational cost of iterative target augmentation, which requires repeatedly conducting inference on the entire training set. While the process of iterative target augmentation may be computationally expensive, we note that it is highly parallelizable, as inference operates independently for each input. Indeed, we leverage this parallelizability in our implementation of iterative target augmentation for the Karel program synthesis task.

\fi
